# Supplementary material for: Infrared phonon anomaly and magnetic excitations in single-crystal Cu$_{3}$Bi(SeO$_{3}$)$_{2}$O$_{2}$Cl
Source: arXiv:1206.1610 source file (2012-10-05)

# Supplementary Information

**Supplementary Figure 1.** The calculated reflectance from the Drude-Lorentz model (red line) superimposed on the measured reflectance (blue points) of $Cu_3Bi(SeO_3)_2O_2Cl$ along the $\hat{b}$ direction at 100 K. Similar qualities of fits were obtained at all other measured polarizations and temperatures.

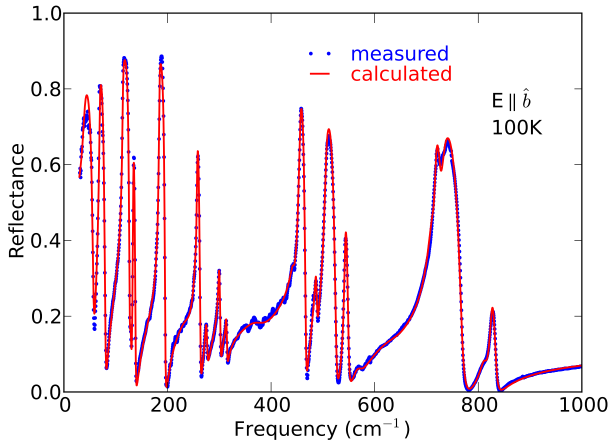


**Supplementary Figure 2.** Rietveld fits of the powder diffraction patterns of $Cu_3Bi(SeO_3)_2O_2Cl$ at 295 K (upper panel) and 85 K (lower panel). (Color online.) Red dots represent data, blue line the Rietveld fit. The difference curve is normalized to the statistical uncertainty of each data point. The fits have $\chi^2$ values of 2.21 (295 K) and 1.70 (85 K). Further details of the refinements are given in the CIF file that accompanies this supplementary information.

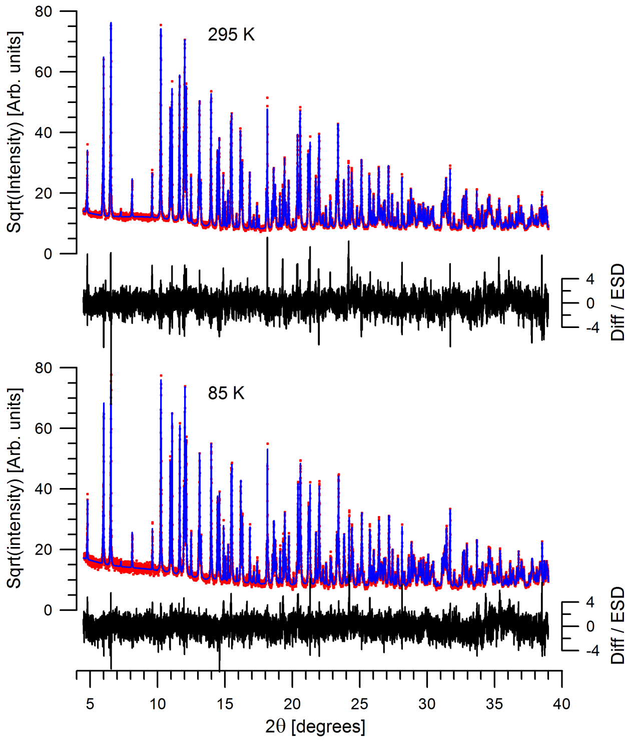

**Supplementary Figure 3.** Field-dependent absorption obtained from the transmitted intensities of four polarizations in the *ab* plane. The external magnetic field was oriented parallel to the *c* axis for all spectra shown.

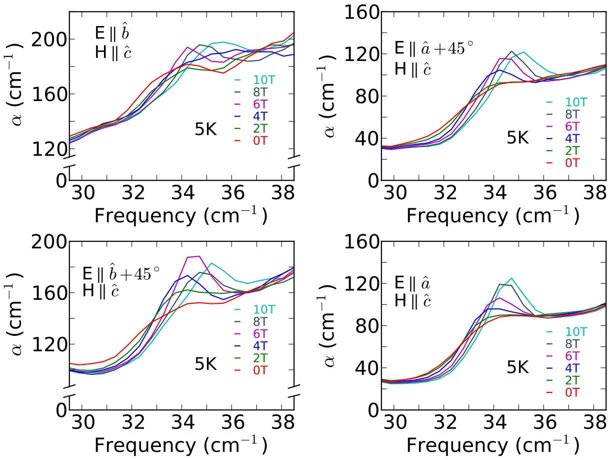

Supplement: Supplementary file 1 [file CBSCl_supinfo_v1.pdf]
